# Supplementary material for: How Privacy-Preserving are Line Clouds? Recovering Scene Details from 3D Lines
Source: arXiv:2103.05086 source file (2021-03-08)
Supplement: Supplementary file 1 [file CvprRebuttal.tex]

\documentclass[rebuttal]{cvpr}

\usepackage{times}
\usepackage{epsfig}
\usepackage{graphicx}
\usepackage{amsmath}
\usepackage{amssymb}
\usepackage{subcaption}
% Include other packages here, before hyperref.

% If you comment hyperref and then uncomment it, you should delete
% egpaper.aux before re-running latex.  (Or just hit 'q' on the first latex
% run, let it finish, and you should be clear).
\usepackage[pagebackref=true,breaklinks=true,colorlinks,bookmarks=false]{hyperref}

%%%%%%%%% PAPER ID  - PLEASE UPDATE
\def\cvprPaperID{****} % *** Enter the CVPR Paper ID here
%\def\httilde{\mbox{\tt\raisebox{-.5ex}{\symbol{126}}}}

\def\cvprPaperID{****} % *** Enter the CVPR Paper ID here
\def\confYear{CVPR 2021}

\begin{document}

%%%%%%%%% TITLE - PLEASE UPDATE
\title{\LaTeX\ Guidelines for Author Response}  % **** Enter the paper title here

\maketitle
\thispagestyle{empty}


%%%%%%%%% BODY TEXT - ENTER YOUR RESPONSE BELOW
\section{Introduction}

After receiving paper reviews, authors may optionally submit a rebuttal to address the reviewers' comments, which will be limited to a {\bf one page} PDF file.  Please follow the steps and style guidelines outlined below for submitting your author response.

Note that the author rebuttal is optional and, following similar guidelines to previous CVPR conferences, it is meant to provide you with an opportunity to rebut factual errors or to supply additional information requested by the reviewers. It is NOT intended to add new contributions (theorems, algorithms, experiments) that were not included in the original submission. You may optionally add a figure, graph or proof to your rebuttal to better illustrate your answer to the reviewers' comments.

Per a passed 2018 PAMI-TC motion, reviewers should not request additional experiments for the rebuttal, or penalize authors for lack of additional experiments. This includes any experiments that involve running code, e.g., to create tables or figures with new results.  \textbf{Authors should not include new experimental results in the rebuttal}, and reviewers should discount any such results when making their final recommendation. Authors may include figures with illustrations or comparison tables of results reported in the submission/supplemental material or in other papers. 

The rebuttal must adhere to the same blind-submission as the original submission and must comply with this rebuttal-formatted template.

%-------------------------------------------------------------------------

\subsection{Response length}
Author responses must be no longer than 1 page in length including any references and figures.  Overlength responses will simply not be reviewed.  This includes responses where the margins and formatting are deemed to have been significantly altered from those laid down by this style guide.  Note that this \LaTeX\ guide already sets figure captions and references in a smaller font.

%------------------------------------------------------------------------
\section{Formatting your Response}

{\bf Make sure to update the paper title and paper ID in the appropriate place in the tex file.}

All text must be in a two-column format. The total allowable width of the text
area is $6\frac78$ inches (17.5 cm) wide by $8\frac78$ inches (22.54 cm) high.
Columns are to be $3\frac14$ inches (8.25 cm) wide, with a $\frac{5}{16}$ inch
(0.8 cm) space between them. The top margin should begin
1.0 inch (2.54 cm) from the top edge of the page.  The bottom margin should be
1-1/8 inches (2.86 cm) from the bottom edge of the page for $8.5 \times
11$-inch paper; for A4 paper, approximately 1-5/8 inches (4.13 cm) from the
bottom edge of the page.

Please number all of your sections and any displayed equations.  It is important
for readers to be able to refer to any particular equation.

Wherever Times is specified, Times Roman may also be used.  Main text should be
in 10-point Times, single-spaced. Section headings should be in 10 or 12 point
Times.  All paragraphs should be indented 1 pica (approx. 1/6 inch or 0.422
cm).  Figure and table captions should be 9-point Roman type as in
Figure~\ref{fig:onecol}.


List and number all bibliographical references in 9-point Times, single-spaced,
at the end of your response. When referenced in the text, enclose the citation
number in square brackets, for example~\cite{Authors14}.  Where appropriate,
include the name(s) of editors of referenced books.

\begin{figure}[t]
\begin{center}
\fbox{\rule{0pt}{1in} \rule{0.9\linewidth}{0pt}}
   %\includegraphics[width=0.8\linewidth]{egfigure.eps}
\end{center}
   \caption{Example of caption.  It is set in Roman so that mathematics
   (always set in Roman: $B \sin A = A \sin B$) may be included without an
   ugly clash.}
\label{fig:long}
\label{fig:onecol}
\end{figure}


%-------------------------------------------------------------------------
\subsection{Illustrations, graphs, and photographs}

All graphics should be centered.  Please ensure that any point you wish to make is resolvable in a printed copy of the response.  Resize fonts in figures to match the font in the body text, and choose line widths which render effectively in print.  Many readers (and reviewers), even of an electronic copy, will choose to print your response in order to read it.  You cannot insist that they do otherwise, and therefore must not assume that they can zoom in to see tiny details on a graphic.

When placing figures in \LaTeX, it's almost always best to use \verb+\includegraphics+, and to specify the  figure width as a multiple of the line width as in the example below
{\small\begin{verbatim}
   \usepackage[dvips]{graphicx} ...
   \includegraphics[width=0.8\linewidth]
                   {myfile.eps}
\end{verbatim}
}


{\small
\bibliographystyle{ieee_fullname}
\bibliography{egbib}
}

\end{document}
